# Supplementary material for: SBNet: Sparse Blocks Network for Fast Inference
Source: arXiv:1801.02108 source file (2018-06-07)
Supplement: Supplementary file 1 [file additional_results.tex]

% !TEX root = ../supplementary.tex
\section{Additional results}

In the main paper, only conv2-conv5 layers were in sparse mode, and the initial convolution,
upsampling, and output layers were still in dense mode. Here, we converted all of the layers to
sparse mode and retrained the sparse network. We provide the speedup and detection accuracy in
Table~\ref{tab:atg4d}. Full sparse networks have much higher average speedup due to the elimination
of all dense layers, while maintaining similar detection accuracy compared to partial sparse
networks. Average overall timings are reported in Table~\ref{tab:mask_overhead}. The full sparse
network with PSP mask reduces the average timing by another 7ms (34.8ms vs. 27.2ms). We also update
the speedup plot in Figure~\ref{fig:full_speedup}.

\begin{table}
\centering
\caption{Speed-up \& detection accuracy of SBNet on the ATG4D dataset. mAP at 70\% IoU.}
\label{tab:atg4d}
\resizebox{0.49\textwidth}{!}{
\begin{small}
\begin{tabular}{|c|c|c|c|c|c|}
\hline
Model       & Sparse        & Train Loss &  Sparsity      & Avg. Speed-up    & mAP         \\
\hline 
Dense       & N/A           & No Mask    &  0\%           & 1.0$\times$      & 74.1        \\  
Dense       & N/A           & Road Mask  &  0\%           & 1.0$\times$      & 75.2        \\
SBNet +Road & conv2-5       & Road Mask  & 75\%           & 1.88$\times$     & \bf{77.2}   \\
SBNet +PSP  & conv2-5       & PSP Mask   & 90\%           & 2.41$\times$     & 73.7        \\
\hline
SBNet +Road & Full          & Road Mask  & 75\%           & 2.03$\times$     & 77.0        \\
SBNet +PSP  & Full          & PSP Mask   & 90\%           & \bf{3.08$\times$}& 73.8        \\
\hline
\end{tabular}
\end{small}
}
\end{table}

\begin{table}
\centering
\caption{Overall network average single forward pass timing and mask network overhead}
\label{tab:mask_overhead}
\begin{small}
\begin{tabular}{|c|c|c|c|}
\hline
Network        & Sparse     & Resolution      & Time (ms)  \\
\hline
Dense          & N/A        & $800\times1408$ & 83.9       \\
\hline
SBNet +Road    & conv2-5  & $800\times1408$ & 44.6       \\
SBNet +PSP     & conv2-5  & $800\times1408$ & 34.8       \\
\hline
SBNet +Road    & Full       & $800\times1408$ & 41.3       \\
SBNet +PSP     & Full       & $800\times1408$ & 27.2       \\
\hline
\hline
PSPNet         & N/A        & $100\times176$  & 3.2        \\
\hline
\end{tabular}
\end{small}
\end{table}

\begin{figure}
\centering
\includegraphics[width=0.9\columnwidth,trim={-1.0cm 0cm 0.0cm 0cm}, clip]{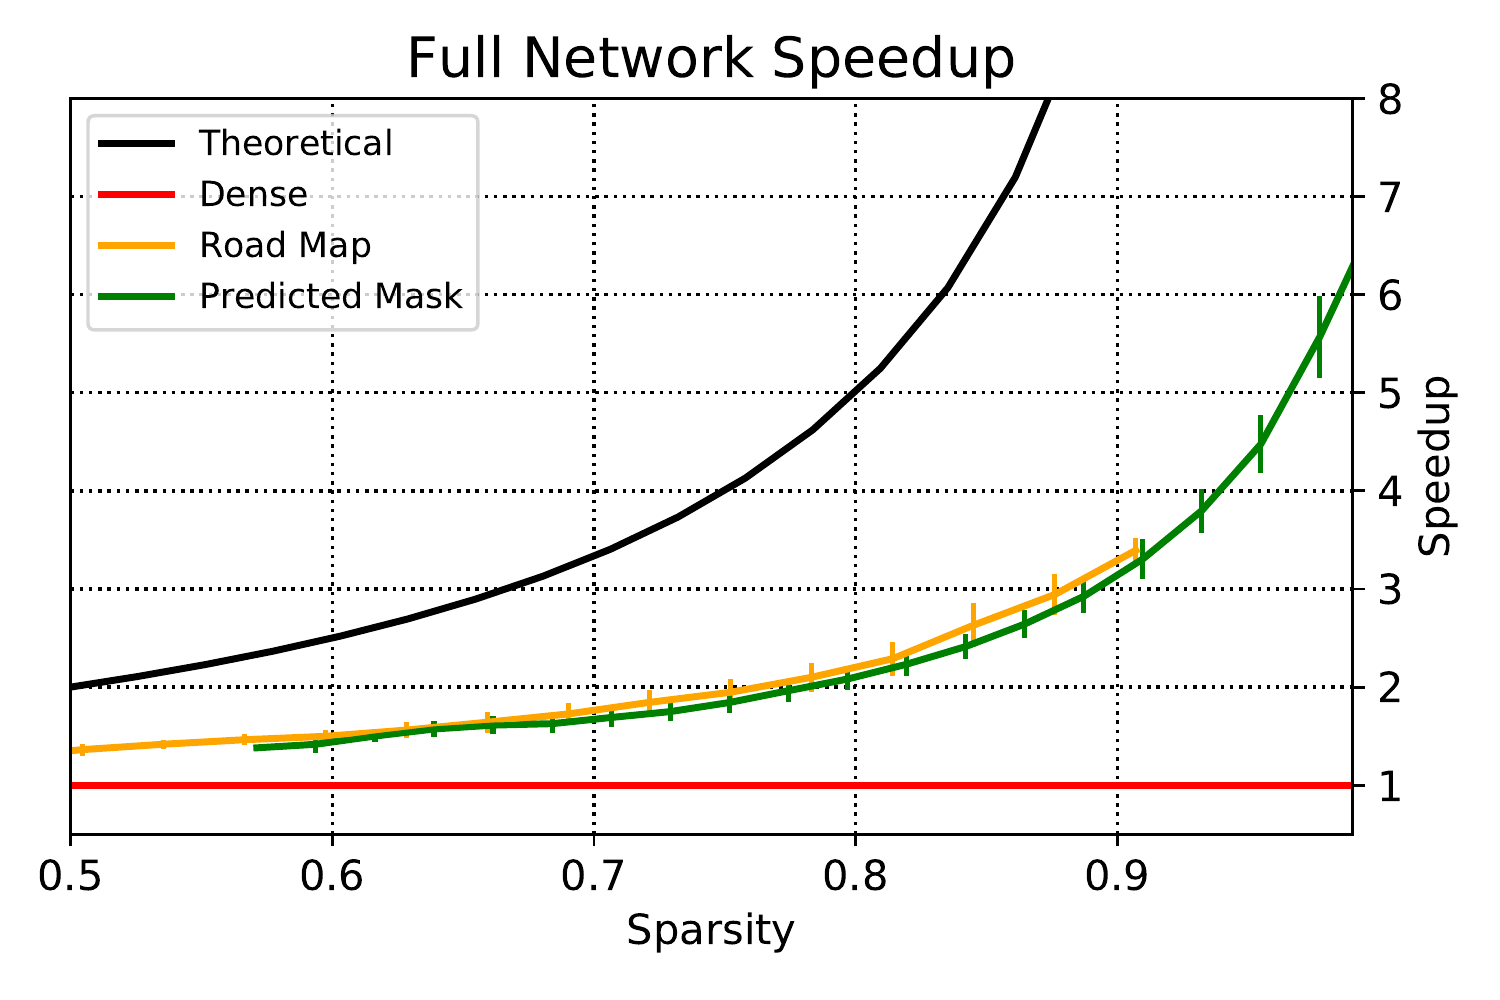}
\caption{
Full detector network speed-ups for using road map and predicted masks.
Individual frames are plotted as scatter points and an average speed-up in each sparsity level is
plotted with standard deviation.
}
\label{fig:full_speedup}
\end{figure}
